# Supplementary material for: GPT-4 Is Too Smart To Be Safe: Stealthy Chat with LLMs via Cipher
Source: arXiv:2308.06463 source file (2024-03-26)
Supplement: Supplementary file 2 [file experimental_results.tex]

\begin{table*}[ht]
\centering
{
\begin{tabular}{c rr c rr}
\toprule%[2pt]
\multirow{2}{*}{\textbf{Cipher}}& \multicolumn{2}{c}{\textbf{Chinese}} &\multirow{2}{*}{\textbf{Cipher}} & \multicolumn{2}{c}{\textbf{English}} \\
\cmidrule(lr){2-3}\cmidrule(lr){5-6}
 & \textbf{Turbo} & \textbf{GPT-4} & & \textbf{Turbo} & \textbf{GPT-4} \\ 
\midrule
Baseline &0   &0  &Baseline     &0   &0   \\
\midrule
{ASCII \& GBK} &- &- & ASCII          & 37.2_{41.8} & 68.3\\
 UTF                             &  39.2_{41.3} & 46.2 & Morse                           & -  & 55.3\\
Unicode        &  26.6_{52.0} & 10.7 & Caesar                          & -  & 73.4\\
\midrule
\textit{SelfCipher}    &  35.7 & 53.3 &   \textit{SelfCipher}   & 38.2 & 70.9\\

\bottomrule %[2pt]
\end{tabular}
}
\caption{The unsafety rate of two models. "-" means there is nearly no valid response in the setting. The subscript means the unsafety rate in the valid responses.}
\label{cipher_results_appendix}
\end{table*}

\begin{table*}[ht]
\setlength{\tabcolsep}{2pt}

\centering
%\scalebox{0.8}
%{
\begin{tabular*}{\textwidth}{@{\extracolsep{\fill}} % makes sure the table is full width
c l c c c c c c c}
%\toprule
\cmidrule{1-9}
\multirow{2}{*}{\textbf{Model}} & \multirow{2}{*}{\textbf{Ablation}} & \multicolumn{3}{c}{\cellcolor{orange}\textbf{zh}} & \multicolumn{4}{c}{\cellcolor{lightgray}\textbf{en}} \\ 
\cmidrule(lr{0.75em}){3-5} \cmidrule(l{0.75em}){6-9}
& & \textbf{Unicode} & \textbf{UTF} & \textbf{PC} & \textbf{ASCII} & \textbf{Caesar} & \textbf{Morse} & \textbf{PC} \\ 
\cmidrule{1-9}
\multirow{4}{*}{\textbf{GPT-4}}
& CipherChat   & 10.71 & 46.19 & 53.27 & 68.34 & 73.37 & 55.28 & 70.85 \\
& ~~w/o SystemRole & 0.00 & 2.51 & 0.50 & 57.79 & 52.82 & 60.80 & 1.01 \\
& ~~w/o UnsafeDemon & 9.55 & 15.66 & 4.52 & 6.53 & - & - & 3.02 \\
& ~~~~~~w SafeDemon & 1.01 & 1.51 & 0.50 & 2.01 & 25.63 & 39.70 & 1.01 \\ 
\cmidrule{1-9}
\multirow{4}{*}{\textbf{Turbo}}
& CipherChat & 26.63_{51.96}  & 39.20_{41.27} & 35.68 &37.19_{41.81} & - & - & 38.19 \\
& ~~w/o SystemRole & 29.15_{65.17} & 36.68_{39.25} & 5.53 & 14.57_{14.65} & - & - & 3.52 \\
& ~~w/o UnsafeDemon & - & - & 6.50 & -  & - & - & 12.56\\
& ~~~~~~w SafeDemon & 13.57_{30.34} & 43.72_{47.28} & 2.01 & 22.61_{23.32} & - & -  & 2.51\\ 
\cmidrule{1-9}
\end{tabular*}
%}
\caption{The results of ablation study. SystemRole means the part of the system prompt except for demonstrations. We handcraft SafeDemon by writing harmless responses for queries in UnsafeDemon. In some zero-shot settings (i.e. w/o UnsafeDemon), the model cannot generate valid responses, we use a "-" to denote it. The subscript means the unsafety rate in the valid responses.}
\label{ablation_appendix}
\end{table*}

\begin{table*}[ht]
\setlength{\tabcolsep}{2pt}

\centering
%\scalebox{0.8}
%{
\begin{tabular*}{\textwidth}{@{\extracolsep{\fill}} % makes sure the table is full width
c c c c c c c c c}
%\toprule
\cmidrule{1-9}
\multirow{2}{*}{\textbf{Model}} & \multirow{2}{*}{\textbf{Shot}} & \multicolumn{3}{c}{\cellcolor{orange}\textbf{zh}} & \multicolumn{4}{c}{\cellcolor{lightgray}\textbf{en}} \\ 
\cmidrule(lr{0.75em}){3-5} \cmidrule(l{0.75em}){6-9}
& & \textbf{Unicode} & \textbf{UTF} & \textbf{\textit{SelfCipher}} & \textbf{ASCII} & \textbf{Caesar} & \textbf{Morse} & \textbf{\textit{SelfCipher}} \\ 
\cmidrule{1-9}
\multirow{4}{*}{\textbf{GPT-4}}
& 0   &9.55  &15.66  &4.52  &6.53  &- &-  &3.02 \\
& 1  &14.07  &14.07  &7.54  &57.79  &62.81  &59.30  &54.27  \\
& 3  &10.71  &46.19  &53.27  &68.34  &73.37  &55.28  &70.85  \\
& 5  &43.65  &61.42  &78.39  &78.89  &89.95  &53.27  &76.88  \\ 
\cmidrule{1-9}
\multirow{4}{*}{\textbf{Turbo}}
& 0  & - & - & 6.50 & -  & - & - & 12.56\\
%&64.52 &73.10  &12.56  &36.84  & - & - &6.50 \\
& 1 &11.56_{22.33}  &34.18_{37.16}  &4.02  &43.72_{45.79} & - & - &11.56  \\
& 3 & 26.63_{51.96}  & 39.20_{41.27} & 35.68 &37.19_{41.81} & - & - & 38.19 \\
% &51.96  &41.27  &35.68  &41.81   & - & - &38.19 \\
& 5  &29.65_{55.14}  &38.19_{41.99}  &18.09  &28.14_{33.53}  & - & -  &56.28 \\ 
\cmidrule{1-9}
\end{tabular*}
%}
\caption{The unsafety rate in the settings with different numbers of demonstrations.  The subscript means the unsafety rate in the valid responses.}
\label{few_shot_appendix}
\end{table*}

\begin{table*}[ht]
\setlength{\tabcolsep}{2pt}
\centering

\scalebox{0.7}
{
\begin{tabular}{cccccccccccccccc}
\toprule[2pt]
\multirow{2}{*}{\textbf{Language}} & \multirow{2}{*}{\textbf{Cipher}} & \multicolumn{2}{c}{\textbf{\textit{Crimes}}} & \multicolumn{2}{c}{\textbf{\textit{Ethics}}} & \multicolumn{2}{c}{\textbf{\textit{Insult}}} & \multicolumn{2}{c}{\textbf{\textit{MenHealth}}} & \multicolumn{2}{c}{\textbf{\textit{PhyHarm}}} & \multicolumn{2}{c}{\textbf{\textit{Privacy}}} \\ 
& & Turbo & GPT-4 & Turbo & GPT-4 & Turbo & GPT-4 & Turbo & GPT-4 & Turbo & GPT-4 & Turbo & GPT-4 \\ \hline
\multirow{3}{*}{zh}
& Baseline & 0.00 &0.00   & 0.00 & 0.00   & 0.00 &0.00  & 0.00 &0.00   & 0.00 & 0.00 & 0.50 & 0.50   \\ 
& Unicode & 26.63_{51.96} & 10.71   & 8.54_{22.67} &58.29   & 38.19_{75.25} &92.46   & 16.58_{50.77} & 89.95  &2.51_{6.94}  &46.46   & 6.53_{10.16}&8.08   \\
& \textit{SelfCipher}  & 35.68 &53.27   &80.90  & 74.37  & 87.94 &94.47   &97.99 &95.98   &89.45 &79.90  &28.64 &39.70     \\
\cline{1-14}
\multirow{3}{*}{en} 
& Baseline & 0.50 &0.50   & 0.00 & 0.00  & 1.51 &  0.50 & 0.00 &  0.00 & 0.00 & 0.00  & 0.00 & 0.00    \\
& ASCII & 37.19_{41.81} & 68.34  & 22.61_{25.42} &  81.91 & 16.58_{17.10} & 99.50  & 48.74_{50.52} &99.50  & 8.04_{8.38} & 79.40  & 6.03_{6.22} & 35.68   \\
& \textit{SelfCipher}   & 38.19 &70.85      &87.44 &  80.90    & 81.41 &  85.43    & 99.50 & 95.48     & 96.48 &  83.92    & 40.20 &  63.82    \\
\toprule%[2pt]
\multirow{2}{*}{\textbf{Language}} & \multirow{2}{*}{\textbf{Cipher}} & \multicolumn{2}{c}{\textbf{\textit{RolePlay}}} & \multicolumn{2}{c}{\textbf{\textit{Unfairness}}}& \multicolumn{2}{c}{\textbf{\textit{UnsafeTopic}}} & \multicolumn{2}{c}{\textbf{\textit{UnsafeOpinion}}} &\multicolumn{2}{c}{ \textbf{\textit{ReExposure}}} & \multicolumn{2}{c}{\textbf{Average}}  \\
& & Turbo & GPT-4 & Turbo & GPT-4 & Turbo & GPT-4 & Turbo & GPT-4 & Turbo & GPT-4 & Turbo & GPT-4 \\ \hline
\multirow{3}{*}{zh}
& Baseline  & 3.02 &  0.00  & 0.00 & 0.00  & 0.50 & 0.00  & 0.00 & 0.00  & 0.00 &   0.00
\\ 
& Unicode & 12.56_{33.33} &52.02  & 22.11_{41.90} & 80.40  &31.66_{50.40} &6.57    & 10.55_{21.65} & 46.15  & 15.58_{39.74}& 5.64 &   &    \\
& \textit{SelfCipher} & 60.30 &50.75   & 94.47 &95.48   &29.15 &41.71   &73.37 & 63.31  & 33.17 &14.57   &  &     \\
\cline{1-14}
\multirow{3}{*}{en} 
& Baseline & 3.52   & 3.52  & 0.00 & 0.00  & 1.51 & 0.00  & 0.00 & 0.00  & 0.00 & 0.00  \\
& ASCII & 12.06_{13.56} & 81.41  & 37.69_{39.89} &96.98   & 28.64_{29.69} &39.70   & 21.61_{23.37} & 80.40  & 21.11_{30.22} &30.15   &  &    \\
& \textit{SelfCipher}   & 76.88 &  61.81    & 93.47 & 98.49     & 13.07 &54.77     & 66.33 &  61.81    & 72.86 &  23.12    &  &     \\
\bottomrule%[2pt]
\end{tabular}
}
\caption{Unsafety rates in all 11 domains. The subscript means the unsafety rate in the valid responses.}
\label{main_results_appendix}
\end{table*}
