# Supplementary material for: GPT-4 Is Too Smart To Be Safe: Stealthy Chat with LLMs via Cipher
Source: arXiv:2308.06463 source file (2024-03-26)
Supplement: Supplementary file 3 [file validity_fluency_accuracy.tex]

\iffalse
\begin{table*}[ht]
\centering
%\renewcommand{\arraystretch}{1.2}
%\scalebox{0.75}
{
\begin{tabular}{ccrrrrrr}
\toprule%[2pt]
\multirow{2}{*}{\textbf{Language}} & \multirow{2}{*}{\textbf{Cipher}} & \multicolumn{2}{c}{\textbf{Validity Rate}} & \multicolumn{2}{c}{\textbf{Fluency}} & \multicolumn{2}{c}{\textbf{Accuracy}} \\ 
& & Turbo & GPT-4  & Turbo & GPT-4& Turbo & GPT-4\\ 
\midrule        
\multirow{6}{*}{Zh}
&Baseline                  &100   &100   &5.0   &5.0   &100.0   &100
\\
& GBK                       &0   &0      &-   &-   &-   &-
\\
& ASCII                     &6   &6    &-   &-   &-   &-
\\
& UTF                       &52   &98   &4.0   &4.7   &88.5   &98.0
\\
&Unicode                   &72   &98     &4.3   &5.0   &91.7   &98.0
\\
& \textit{SelfCipher}               &100   &100     &5.0   &5.0   &96.0   &98.0
\\
\hline
\multirow{6}{*}{En}
&Baseline                  &100   &100    &5.0   &5.0   &100.0  &100.0\\
& Caesar                    &0   &94    &-   &2.9   &-   &100.0\\
& Atbash                    &0   &24     &-   &1.8   &-   &91.7
\\
& Morse                     &0   &86     &-   &4.5   &-   &100.0\\
&ASCII                    &48   &100     &3.3   &5.0   &79.2   &98.0
\\
& \textit{SelfCipher}               &100   &100       &5.0   &5.0   &100.0   &97.9
\\ 
\bottomrule %[2pt]
\end{tabular}
}
\caption{"Validity rate" represents the proportion of valid responses. "Fluency" is obtained from GPT-4, rating from 1 (worst) to 5 (best). "Accuracy" is the accuracy of the GPT-4-based unsafety detector.}
\label{valid_rate_appendix}
\end{table*}
\fi

\begin{table*}
\centering
{
\begin{tabular}{c rr c rr}
\toprule%[2pt]
\multirow{2}{*}{\textbf{Cipher}}& \multicolumn{2}{c}{\textbf{Chinese}} &\multirow{2}{*}{\textbf{Cipher}} & \multicolumn{2}{c}{\textbf{English}} \\
\cmidrule(lr){2-3}\cmidrule(lr){5-6}
 & \textbf{Turbo} & \textbf{GPT-4} & & \textbf{Turbo} & \textbf{GPT-4} \\ 
\midrule
Baseline         &  100.0   & 100.0  & Baseline     & 100.0   &  100.0 \\
\midrule
{ASCII \& GBK}   &  -       &  -     & ASCII        & 79.2    &   98.0\\
 UTF             &   88.5   &  98.0  & Morse        & -       &  100.0\\
Unicode          &   91.7   &  98.0  & Caesar       & -       &  100.0\\
\midrule
\textit{SelfCipher}    &  96.0 & 98.0 &   \textit{SelfCipher}   & 100.0 & 97.9\\

\bottomrule %[2pt]
\end{tabular}
}
\caption{Accuracy of the GPT-4-based unsafety detector.}
\label{human_evaluation_detection}
\end{table*}

\begin{table*}[ht]
\centering
\scalebox{0.8}
{
\begin{tabular}{cccccccccccc}
\toprule%[2pt]
\multirow{2}{*}{\textbf{Language}} & \multirow{2}{*}{\textbf{Cipher}} & \multicolumn{2}{c}{\textbf{WrongCipher}}  & \multicolumn{2}{c}{\textbf{Unnatural}} & \multicolumn{2}{c}{\textbf{RepeatQuery}} & \multicolumn{2}{c}{\textbf{RepeatDemon}}& \multicolumn{2}{c}{\textbf{UnrelatedAns}} \\
& & Turbo & GPT-4  & Turbo & GPT-4& Turbo & GPT-4& Turbo & GPT-4 &Turbo & GPT-4\\
\midrule
\multirow{6}{*}{zh}
&Baseline                   &0   &0   & 0  & 0   & 0  &0   & 0  &0  & 0  &0
\\
& GBK                       & 6  & 1  &  0 &  1  & 34  & 30  & 10  &18  & 0  &0
\\
& ASCII                     & 25  &  1 &   0&   10 & 21  &  29 & 1  &3&  5 &4
\\
& UTF                       & 3    &   1&   4&  0  &   15&  0 &   0&0&   0   &0
\\
&Unicode                   &   0&  0 &  7 &   1 &   6& 0  &  0 &0&   1  &0
\\
&\textit{SelfCipher}               &  0 &  0 & 0  &  0  & 0  &  0 & 0  &0&  0   &0
\\
\midrule
\multirow{6}{*}{en}
&Baseline                  &0   &1   &0   & 0   & 0  &1   &  0 &0&   0  &0
\\
& Caesar                    & 35  & 0  &   2&  0  & 11  & 2  & 2  &0&  0   &1
\\
& Atbash                    &  21 &  0 &  4 &   9 &   20&  16 & 0  &7&  5      &6
\\  
& Morse                     &  50 &   0& 0  &  0  &  0 & 7  & 0  &0&  0   &0
\\
&ASCII                     &  1 &   0&   0& 0   & 17  & 0  &2   &0&   6  &0
\\
&\textit{SelfCipher}               & 0  &   0&   0&  0  & 0  &  0 & 0  &0&     0&0
\\
\bottomrule %[2pt]
\end{tabular}
}
\caption{The number of invalid responses for each cipher. The total number of responses in each setting is 50.}
\label{invalid_appendix}
\end{table*}
